# Supplementary material for: Parameter Expanded Stochastic Gradient Markov Chain Monte Carlo
Source: arXiv:2503.00699 source file (2025-03-02)
Supplement: Supplementary file 1 [file scribble.tex]

\clearpage
\newpage
\section{Scribbles}

\begin{table}[ht]
    \centering
    \caption{bla}
    \begin{tabular}{cccccc}
    \toprule
    $m$ & $\lambda$ & ERR & NLL & AMB \\
    \midrule
    1.0 & 1.0 & \\
        & 2.0 & \\
        & 5.0 & \\
        & 10. & \\
    \midrule
    0.5 & 1.0 & .115 & .369 & .254 \\
        & 2.0 & .116 & .371 & .247 \\
        & 5.0 & .119 & .381 & .220 \\
        & 10. & \\
    \midrule
    0.0 & 1.0 \\
        & 2.0 \\
        & 5.0 \\
        & 10. \\
    \bottomrule
    \end{tabular}
\end{table}

\begin{table}[ht]
    \centering
    \caption{From scratch. $\log{p(\bQ)} = \lambda \cdot \norm{\bQ\bQ\tr - m\bI}_{F}^{\alpha}$.}
    \begin{tabular}{ccccccl}
    \toprule
    $m$ & $\alpha$ & $\lambda$ & EnsERR & EnsNLL & EnsAMB & Label \\
    \midrule
    1.0 & 0.5 & 10. & .132 & .419 & .263 \\
        & 1.0 & 2.0 & .125 & .405 & .234 & QSGHMC (Orth) \\
        & 1.5 & 2.0 & .131 & .420 & .205 \\
        & 2.0 & 1.0 & .140 & .443 & .187 \\
        & 2.5 & 1.0 & .153 & .480 & .174 \\
    0.5 & 0.5 & 10. & .133 & .428 & .269 \\
        & 1.0 & 1.0 & \BF{.121} & \BF{.391} & .232 \\
        & 1.5 & 2.0 & .133 & .418 & .203 \\
        & 2.0 & 1.0 & .140 & .446 & .186 \\
        & 2.5 & 1.0 & .159 & .512 & .166 \\
    0.0 & 0.5 & 10. & .133 & .427 & \BF{.271} \\
        & 1.0 & 2.0 & .126 & .402 & .230 \\
        & 1.5 & 1.0 & .131 & .419 & .213 \\
        & 2.0 & 1.0 & .137 & .440 & .183 \\
        & 2.5 & 1.0 & .163 & .521 & .172 \\
    \bottomrule
    \end{tabular}
\end{table}

\subsection{Orthogonality regularization}

\begin{itemize}
\item \[
    \norm{\bQ\bQ\tr - \bI}_{F} \rightarrow 0
\]
\item \[
    \frac{\norm{\bQ\bQ\tr - \bI_{d}}_{F}}{\sqrt{d}} \rightarrow 0
\]
\item \[
    \norm{\bQ\bQ\tr - \bI}_{2}
    = \sigma_{\text{max}} (\bQ\bQ\tr - \bI) \rightarrow 0.
\]
\item \[
    \bsu \gets (\bQ\bQ\tr - \bI) \bsv, \quad
    \bsv \gets (\bQ\bQ\tr - \bI) \bsu, \quad
    \sigma_{\text{max}} (\bQ\bQ\tr - \bI) \gets \frac{\norm{\bsv}}{\norm{\bsu}}.
\]
\end{itemize}

% \[
% \norm{\bQ}_{F}^{2} = \Tr{\left( \bQ\bQ\tr \right)}
% \]

% \[
% \bQ = \bU\bSigma\bV\tr
% \]

% \[
% \bQ\bQ\tr
% = \left( \bU\bSigma\bV\tr \right) \left( \bU \bSigma\bV\tr \right)\tr
% = \bU \bSigma^2 \bU\tr
% \]

\[
\norm{\bQ\bQ\tr - \bI}_{F}
= \norm{\bSigma^{2} - \bI}_{F}
= \sqrt{\sum_{i=1}^{r} (\sigma_{i}^{2} - 1)^{2}}
\]

\[
\left\lVert \bQ\bQ\tr / \norm{\bQ}_{F}^{2} - \bI \right\rVert_{F}
= \norm{\frac{\bSigma^{2}}{\norm{\bQ}_{F}^{2}} - \bI}_{F}
= \norm{\frac{\bSigma^{2}}{\sum_{i=1}^{r} \sigma_{i}^{2}} - \bI}_{F}
= \sqrt{\sum_{i=1}^{r} (\frac{\sigma_{i}^{2}}{\sum_{j} \sigma_{j}^{2}} - 1)^{2}}
\]

{\color{purple}
\textbf{Conjecture.}
Regularizing $\norm{\bQ}_{F}^{2}$ is better than regularizing $\norm{\bQ\bQ\tr - \bI}_{F}^{2}$.

\[
\norm{\bQ}_{F}^{2}
= \sum_{i=1}^{r} \sigma_{i}^{2}, \quad
\norm{\bQ\bQ\tr - \bI}_{F}^{2}
= \sum_{i=1}^{r} \left( \sigma_{i}^{2} - 1 \right)^{2}.
\]

\textbf{Remark \#1.}
$\norm{\bQ}_{F}^{2}$ pushes the singular values towards zero, while $\norm{\bQ\bQ\tr - \bI}_{F}^{2}$ encourages the singular values to move closer to plus-minus-one.

\textbf{Remark \#2.}
Since we initialize $\bQ$ as the identity matrix, it initially acts like an orthogonal matrix.
However, as the singular values decrease towards zero, $\bQ$ loses this property, distorting its ability to preserve some geometric relationships in the parameter space.

\textbf{Remark \#3.}
Rank deficiency; it collapses part of the space into a lower dimension? MCMC dynamics in the subspace? removes unimportant / less significant information?
}

\[
\norm{\bQ\bQ\tr - \bI}_{F}^{2}
= \norm{\bU \bSigma^2 \bU\tr - \bI}_{F}^{2}
= \norm{\bSigma^{2} - \bI}_{F}^{2}
= \sum_{i=1}^{r} \left( \sigma_{i}^{2} - 1 \right)^{2}
\]

\[
\norm{\bQ\bQ\tr - \bI}_{F}^{2} - \norm{\bQ}_{F}^{2}
= \sum_{i=1}^{r} \left( \sigma_{i}^{2} - 1 \right)^{2} - \sum_{i=1}^{r} \sigma_{i}^{2}
= \sum_{i=1}^{r} \left( \sigma_{i}^{4} - 3\sigma_{i}^{2} + 1 \right)
\]

\begin{enumerate}
    \item SGHMC : $\underbrace{\bW_2}_{D_3 \times D_2} \sigma\left( \underbrace{\bW_1}_{D_2 \times D_1} \underbrace{\bsx}_{D_1 \times 1} \right)$
    \item v13 : $\underbrace{\bW_2}_{D_3 \times D_2} \underbrace{\bQ\tr}_{D_2 \times D_2} \sigma\left( \underbrace{\bQ}_{D_2 \times D_2} \underbrace{\bW_1}_{D_2 \times D_1} \underbrace{\bsx}_{D_1 \times 1} \right)$
    \item v13-side $\underbrace{\bW_2}_{D_3 \times D_2} \underbrace{\bQ\tr}_{D_2 \times D_2} \sigma\left( \underbrace{\bW_1}_{D_2 \times D_1} \underbrace{\bsx}_{D_1 \times 1} \right)$
    \item v13-q1q2 : $\underbrace{\bW_2}_{D_3 \times D_2} \underbrace{\bQ_2}_{D_2 \times D_2} \sigma\left( \underbrace{\bQ_1}_{D_2 \times D_2} \underbrace{\bW_1}_{D_2 \times D_1} \underbrace{\bsx}_{D_1 \times 1} \right)$
    \item v13-q1q2-rank4 : $\underbrace{\bW_2}_{D_3 \times D_2} \left( \underbrace{\bR_2}_{D2 \times 4} \underbrace{\bS_2}_{4 \times D_2} \right) \sigma\left( \left(\underbrace{\bR_1}_{D_2 \times 4} \times \underbrace{\bS_2}_{4 \times D_2} \right) \underbrace{\bW_1}_{D_2 \times D_1} \underbrace{\bsx}_{D_1 \times 1} \right)$
\end{enumerate}

\begin{table}[ht]
    \centering
    \caption{\textbf{Validation results for SGHMC on CIFAR-10.}}
    \begin{tabular}{lccccc}
    \toprule
    & \multicolumn{2}{c}{Priors} & \multicolumn{3}{c}{Evaluation metrics} \\
    \cmidrule(lr){2-3}\cmidrule(lr){4-6}
    Parameterization & $p(\bW)$ & $p(\bQ)$ & ERR & NLL & AMB \\
    \midrule
    $\bW_{2} \phantom{\bQ_{\phantom{2}}\tr} \sigma\left( \phantom{\bQ_{\phantom{1}}}\bW_{1}\bsx \right)$
        & L2 & -    & .132\PM{.004} & .417\PM{.004} & .186\PM{.004} \\
    \midrule
    $\bW_{2} \phantom{\bQ_{\phantom{2}}\tr} \sigma\left( \phantom{\bQ_{\phantom{1}}}\bW_{1}\bsx \right)$
        & L2 & -    & .135\PM{.005} & .444\PM{.007} & .196\PM{.004} \\
    $\bW_{2} \bQ_{\phantom{2}}\tr \sigma\left( \phantom{\bQ_{\phantom{1}}}\bW_{1}\bsx \right)$
        & L2 & L2   & .127\PM{.002} & .404\PM{.004} & .215\PM{.004} \\
        & L2 & Orth & .127\PM{.000} & .405\PM{.003} & .208\PM{.001} \\
    $\bW_{2} \bQ_{\phantom{2}}\tr \sigma\left( \bQ_{\phantom{1}}\bW_{1}\bsx \right)$
        & L2 & L2   & .125\PM{.003} & .401\PM{.004} & .231\PM{.002} \\
        & L2 & Orth & .125\PM{.002} & .398\PM{.002} & .234\PM{.004} \\
    $\bW_{2} \bQ_{2}\tr \sigma\left( \bQ_{1}\bW_{1}\bsx \right)$
        & L2 & L2   & .116\PM{.003} & .369\PM{.005} & .254\PM{.001} \\
        & L2 & Orth & \\
    \bottomrule
    \end{tabular}
\end{table}

\begin{table}[ht]
    \centering
    \caption{\textbf{Validation results for SGHMC on CIFAR-10.}}
    \begin{tabular}{lccccc}
    \toprule
    & \multicolumn{2}{c}{Priors} & \multicolumn{3}{c}{Evaluation metrics} \\
    \cmidrule(lr){2-3}\cmidrule(lr){4-6}
    Parameterization & $p(\bW)$ & $p(\bQ)$ & ERR & NLL & AMB \\
    \midrule
    HMC & - & - & .122 & .382 & .360 \\
    \midrule
    $\bW_{2} \phantom{\bQ_{\phantom{2}}\tr} \sigma\left( \phantom{\bQ_{\phantom{1}}}\bW_{1}\bsx \right)$
        & L2 & -    & .158 & .498 & .138 \\
    $\bW_{2} \bQ_{\phantom{2}}\tr \sigma\left( \phantom{\bQ_{\phantom{1}}}\bW_{1}\bsx \right)$
        & L2 & L2   & .138 & .410 & .190 \\
    $\bW_{2} \bQ_{\phantom{2}}\tr \sigma\left( \bQ_{\phantom{1}}\bW_{1}\bsx \right)$
        & L2 & L2   & .137 & .414 & .221 \\
    $\bW_{2} \bQ_{2}\tr \sigma\left( \bQ_{1}\bW_{1}\bsx \right)$
        & L2 & L2   & .122 & .375 & .307 \\
    \bottomrule
    \end{tabular}
\end{table}

\begin{table}[ht]
    \centering
    \caption{\textbf{Validation results for SGNHT on CIFAR-10.}}
    \begin{tabular}{lccccc}
    \toprule
    & \multicolumn{2}{c}{Priors} & \multicolumn{3}{c}{Evaluation metrics} \\
    \cmidrule(lr){2-3}\cmidrule(lr){4-6}
    Parameterization & $p(\bW)$ & $p(\bQ)$ & ERR & NLL & AMB \\
    \midrule
    $\bW_{2} \phantom{\bQ\tr} \sigma\left( \phantom{\bQ}\bW_{1}\bsx \right)$
        & L2 & -    & .136\PM{.002} & .447\PM{.005} & .197\PM{.002} \\
    $\bW_{2} \bQ\tr \sigma\left( \phantom{\bQ}\bW_{1}\bsx \right)$
        & L2 & L2   & \\
        & L2 & Orth & \\
    $\bW_{2} \bQ\tr \sigma\left( \bQ\bW_{1}\bsx \right)$
        & L2 & L2   & \\
        & L2 & Orth & .124\PM{.003} & .400\PM{.007} & .231\PM{.003} \\
    \bottomrule
    \end{tabular}
\end{table}

\begin{figure} % temporary; to avoid warnings...
    \centering
    \begin{subfigure}[b]{0.3\textwidth}
        \centering
        \caption{$y=x$}
    \end{subfigure}
\end{figure}
