# Supplementary material for: Parameter Expanded Stochastic Gradient Markov Chain Monte Carlo
Source: arXiv:2503.00699 source file (2025-03-02)
Supplement: Supplementary file 2 [file theorem.tex]

\section{Proofs}
\label{app:proof2}

\begin{thm}
    With the parameter initialization of \citet{arora2018on} for both $\btheta$ and $\br$, the expectation of acceptance probability in GGMC \citep{alonso2021exact}, whose special case is SGHMC, is bounded
\end{thm}
\begin{proof}
\[
    \bZ(t) = \begin{bmatrix}
        \bW_{1:e}(t),\\
        \bU_{1:e}(t)
    \end{bmatrix},
    \bY = \V{\bZ^{l}}_{l=1}^L
\]
\[
    \frac{\dee H}{\dee t}&= \left<\frac{\partial H}{\partial \bY(t)},\frac{\dee \bY(t)}{\dee t}\right>\\
    &=\sum_{l=1}^L\left<\nabla_{\bY\lyr{l}} H(\bY\lyr{l}(t)),-(\bD+\bQ)P_{\bY(t)}\nabla_{\bY\lyr{l}}H(\bY\lyr{l}(t))+\bzeta\lyr{l}\right>\\
    &\leq -\lambda_\text{min}(\bD+\bQ)\Sigma_\text{min}^{2(e-1)/e}\sum_{1=1}^L\norm{\nabla_{\bY\lyr{l}}H}^2_F + \sum_{1=1}^L\left<\nabla_{\bY\lyr{l}}H,\bzeta\lyr{l}\right>,
\] where $\bD$ and $\bQ$ are the drift matrices defined as in GGMC~\citet{alonso2021exact}. 
\[
\bbE[-H(t+1) + H(t)] \leq -\lambda_\text{min}(\bD+\bQ)\Sigma_\text{min}^{2(e-1)/e}\sum_{1=1}^L\bbE[\norm{\nabla_{\bY\lyr{l}}H}^2_F]
\] Due to the convexity of $\exp$,
\[
\bbE[\text{AcceptProb}] &= \bbE[\exp(-H(t+1) + H(t))]\\
&\geq \exp(\bbE[-H(t+1) + H(t)])\\
&\geq \exp\left(\frac{\epsilon_t}{T}\lambda_\text{min}(\bD+\bQ)\Sigma_\text{min}^{2(e-1)/e}\sum_{1=1}^L\bbE[\norm{\nabla_{\bY\lyr{l}}H}^2_F]\right).
\]
\end{proof}
